# Supplementary material for: Discriminative and Generative Transformer-based Models For Situation Entity Classification
Source: arXiv:2109.07434 source file (2021-09-15)
Supplement: Supplementary file 1 [file additional_experiments.tex]

\begin{table}[]
    \centering
    \scalebox{0.8}{        
    \begin{tabular}{l|cccc}
    \specialrule{.1em}{.05em}{.05em} 
    Genre     & Context Aware & Bert & Par Bert&LSTM Par Bert    &Humans \\ \hline
    blog      & 70.3       &\textbf{72.03}&74.14&72.68 & 72.9 \\
    email     & 71.5       &\textbf{73.84}&75.88&74.95 & 67.0 \\
    essays    & 64.1       &\textbf{66.99}&67.49&66.67 & 64.6 \\
    ficlets   & 68.8       &\textbf{75.14}&73.11&73.20 & 81.7 \\
    fiction   & 72.1       &\textbf{77.52}&75.42&77.28 & 76.7 \\ 
    gov-docs  & 68.9       &\textbf{72.52}&72.31&71.04 & 72.6\\
    jokes     & 75.0       &\textbf{77.11}&74.46&76.38 & 82.0\\
    journal   & 66.4       &\textbf{68.75}&68.81&70.68& 63.7\\
    letters   & 71.2       &\textbf{72.01}&75.64&74.07 & 68.0\\
    news      & 72.7       &\textbf{75.20}&74.58&76.42& 78.6\\
    technical & 60.5       &\textbf{61.72}&53.38&65.29&54.7\\
    travel    & 53.6       &\textbf{68.54}&54.74&58.28& 48.9\\
    wiki      & 60.6       &\textbf{63.04}&64.58&66.16& 69.2\\
    \specialrule{.1em}{.05em}{.05em} 
    \end{tabular}
    }
    \caption{Cross-genre Classification Results by Genre on the Training Set of MASC+Wiki.}
    \label{cross-genre result by genre}
\end{table}  

    \begin{table}[]
        \centering
        \begin{tabular}{l|ccc}
        \specialrule{.1em}{.05em}{.05em} 
        Genre     & Context Aware & Bert    &Humans \\ \hline
        blog      & 70.3       &\textbf{72.03} & 72.9 \\
        email     & 71.5       &\textbf{73.84} & 67.0 \\
        essays    & 64.1       &\textbf{66.99} & 64.6 \\
        ficlets   & 68.8       &\textbf{75.14}  & 81.7 \\
        fiction   & 72.1       &\textbf{77.52}  & 76.7 \\ 
        gov-docs  & 68.9       &\textbf{72.52} & 72.6\\
        jokes     & 75.0       &\textbf{77.11} & 82.0\\
        journal   & 66.4       &\textbf{68.75} & 63.7\\
        letters   & 71.2       &\textbf{72.01} & 68.0\\
        news      & 72.7       &\textbf{75.20} & 78.6\\
        technical & 60.5       &\textbf{61.72}& 54.7\\
        travel    & 53.6       &\textbf{68.54} & 48.9\\
        wiki      & 60.6       &\textbf{63.04} & 69.2\\
        \specialrule{.1em}{.05em}{.05em} 
        \end{tabular}
        \caption{Cross-genre Classification F-1 Scores by Genre on the Training Set of MASC+Wiki.}
        \label{cross-genre result by genre}
    \end{table}
    
    \begin{figure*}
    \centering
        \begin{subfigure}[b]{0.32\textwidth}
        \includegraphics[width=\textwidth]{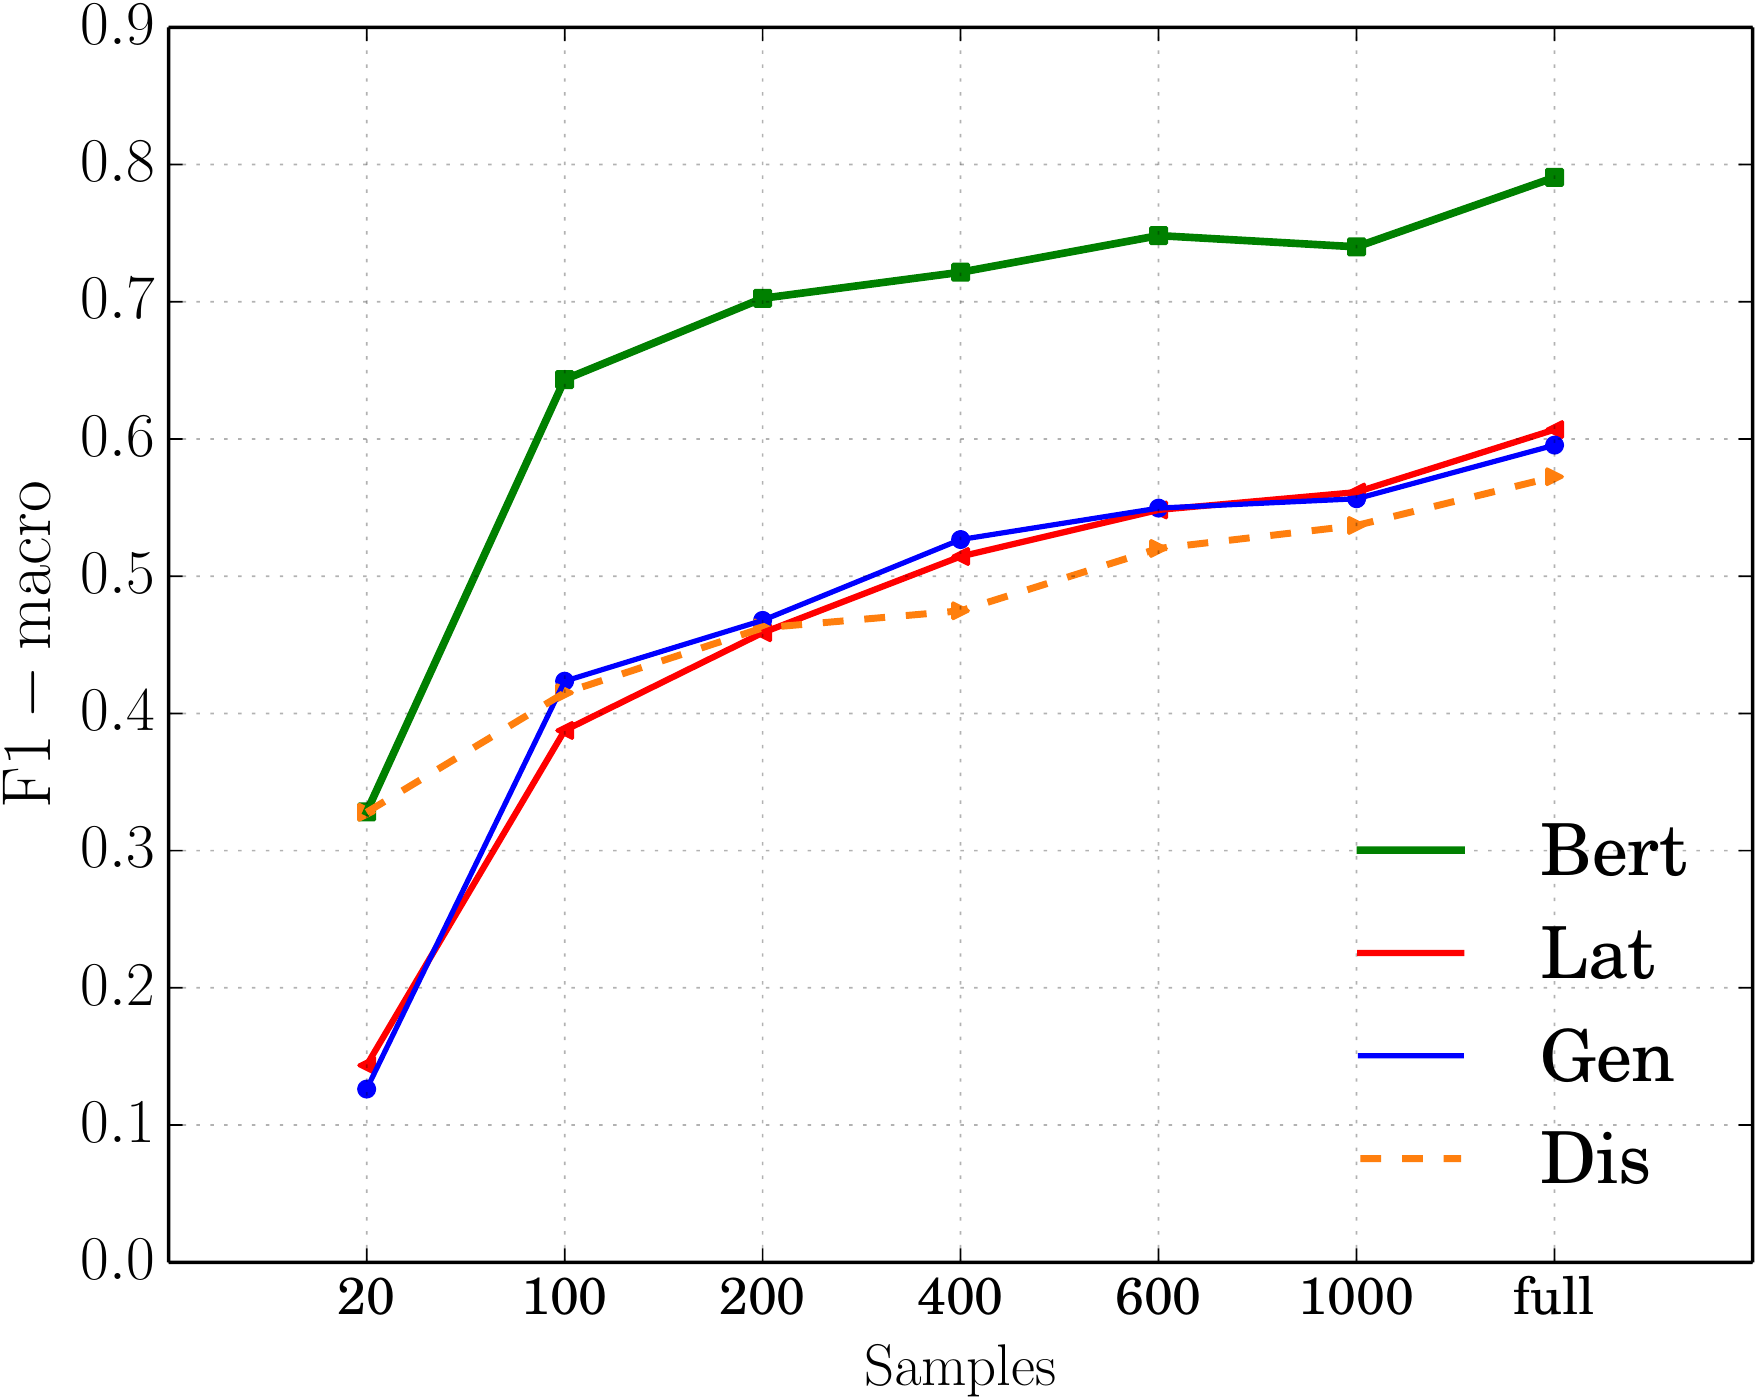}
        \caption{F1-macro}
        \label{fig:tiger}
    \end{subfigure}
    ~ %add desired spacing between images, e. g. ~, \quad, \qquad, \hfill etc. 
      %(or a blank line to force the subfigure onto a new line)
    \begin{subfigure}[b]{0.32\textwidth}
        \includegraphics[width=\textwidth]{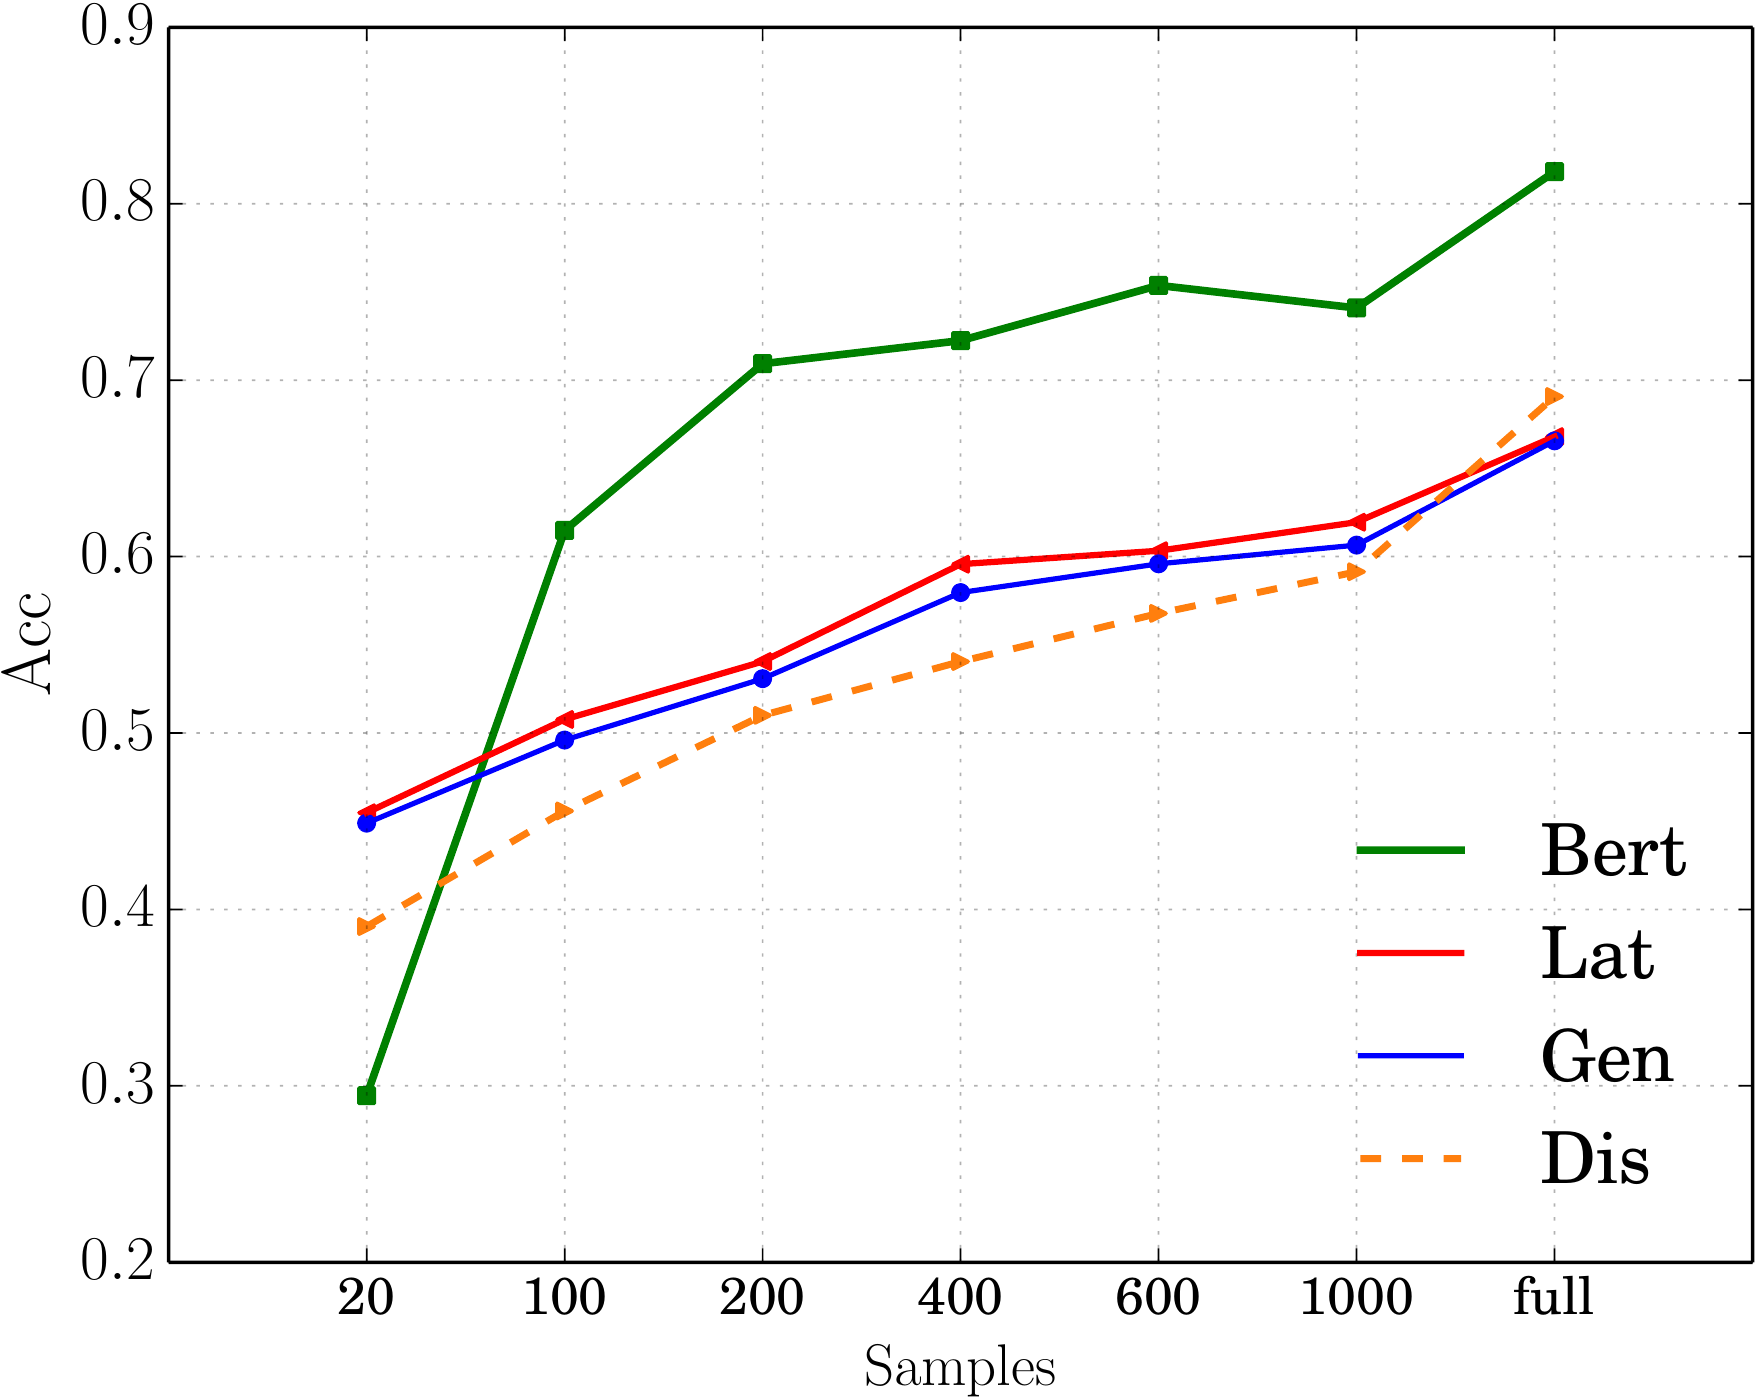}
        \caption{Accuracy}
        \label{fig:gull}
    \end{subfigure}
    ~ %add desired spacing between images, e. g. ~, \quad, \qquad, \hfill etc. 
    %(or a blank line to force the subfigure onto a new line)
    \begin{subfigure}[b]{0.32\textwidth}
        \includegraphics[width=\textwidth]{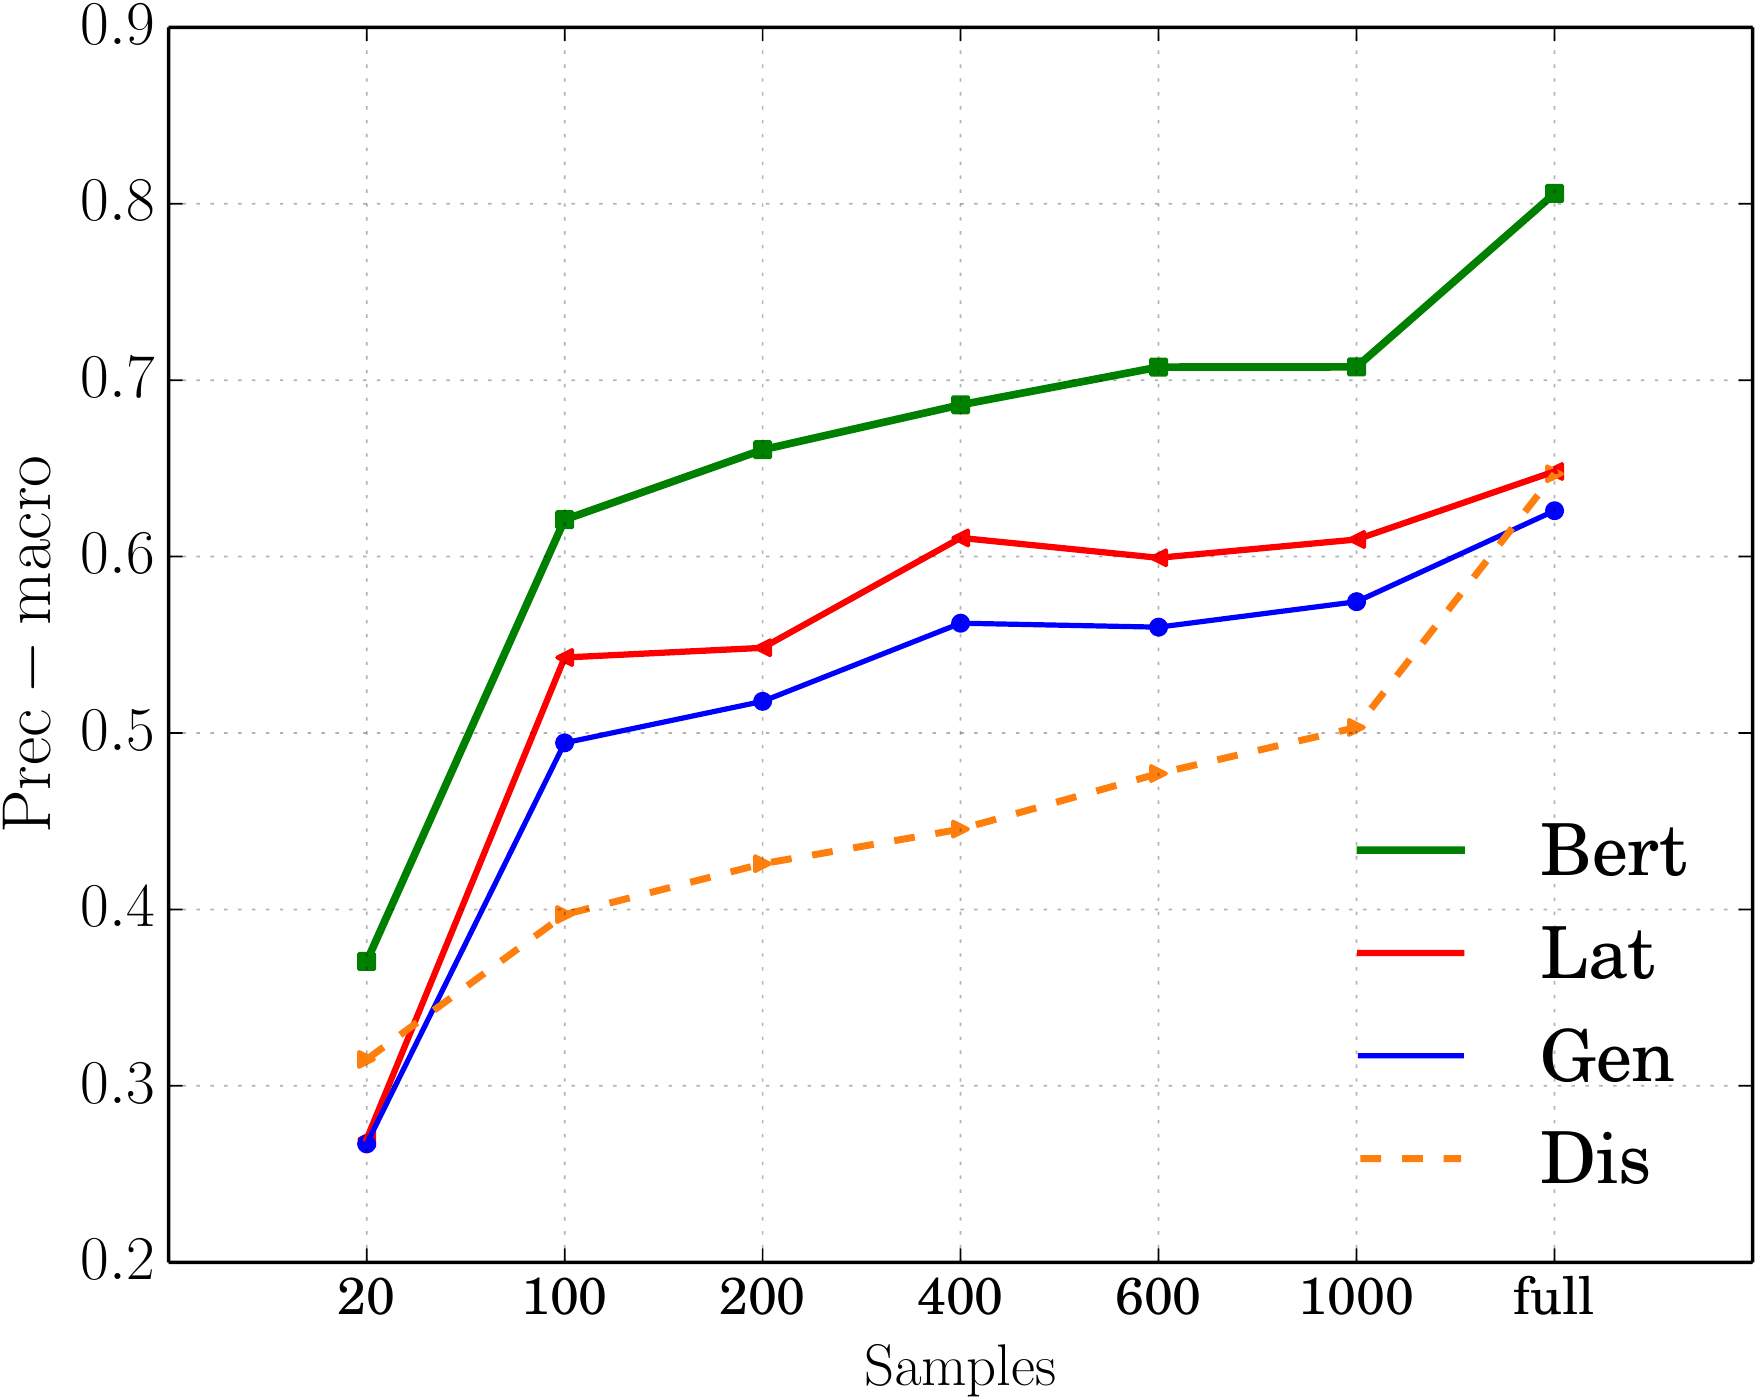}
        \caption{precision-macro}
        \label{fig:mouse}
    \end{subfigure}
\end{figure*}
\begin{table}[]
    \centering
    \scalebox{0.72}{        
    \begin{tabular}{l|ccccc}
    \specialrule{.1em}{.05em}{.05em} 
    Genre     & Context Aware & Bert & Par Bert & OptCls    &Humans \\ \hline
    blog      & 70.3       &{72.03}  & 74.14 & 72.37  & 72.9 \\
    email     & 71.5       &{73.84}  & 75.88 & 74.53  & 67.0 \\
    essays    & 64.1       &{66.99}  & 67.49 & 66.15  & 64.6 \\
    ficlets   & 68.8       &{75.14}  & 73.11 & 73.86  & 81.7 \\
    fiction   & 72.1       &{77.52}  & 75.42 & 78.99  & 76.7 \\ 
    gov-docs  & 68.9       &{72.52}  & 72.31 & 71.08  & 72.6 \\
    jokes     & 75.0       &{77.11}  & 74.46 & 76.73  & 82.0 \\
    journal   & 66.4       &{68.75}  & 68.81 & 71.96  & 63.7 \\
    letters   & 71.2       &{72.01}  & 75.64 & 71.93  & 68.0 \\
    news      & 72.7       &{75.20}  & 74.58 & 73.11  & 78.6 \\
    technical & 60.5       &{61.72}  & 53.38 & 62.72  & 54.7 \\
    travel    & 53.6       &{68.54}  & 54.74 & 58.18  & 48.9 \\
    wiki      & 60.6       &{63.04}  & 64.58 & 67.86  & 69.2 \\
    \specialrule{.1em}{.05em}{.05em} 
    \end{tabular}
    }
    \caption{Cross-genre Classification Results by Genre on the Training Set of MASC+Wiki.}
    \label{cross-genre-result-by-genre-sorted}
\end{table}  
% \begin{figure*}[t!]
%   \centering
%   \includegraphics[width=0.8\linewidth]{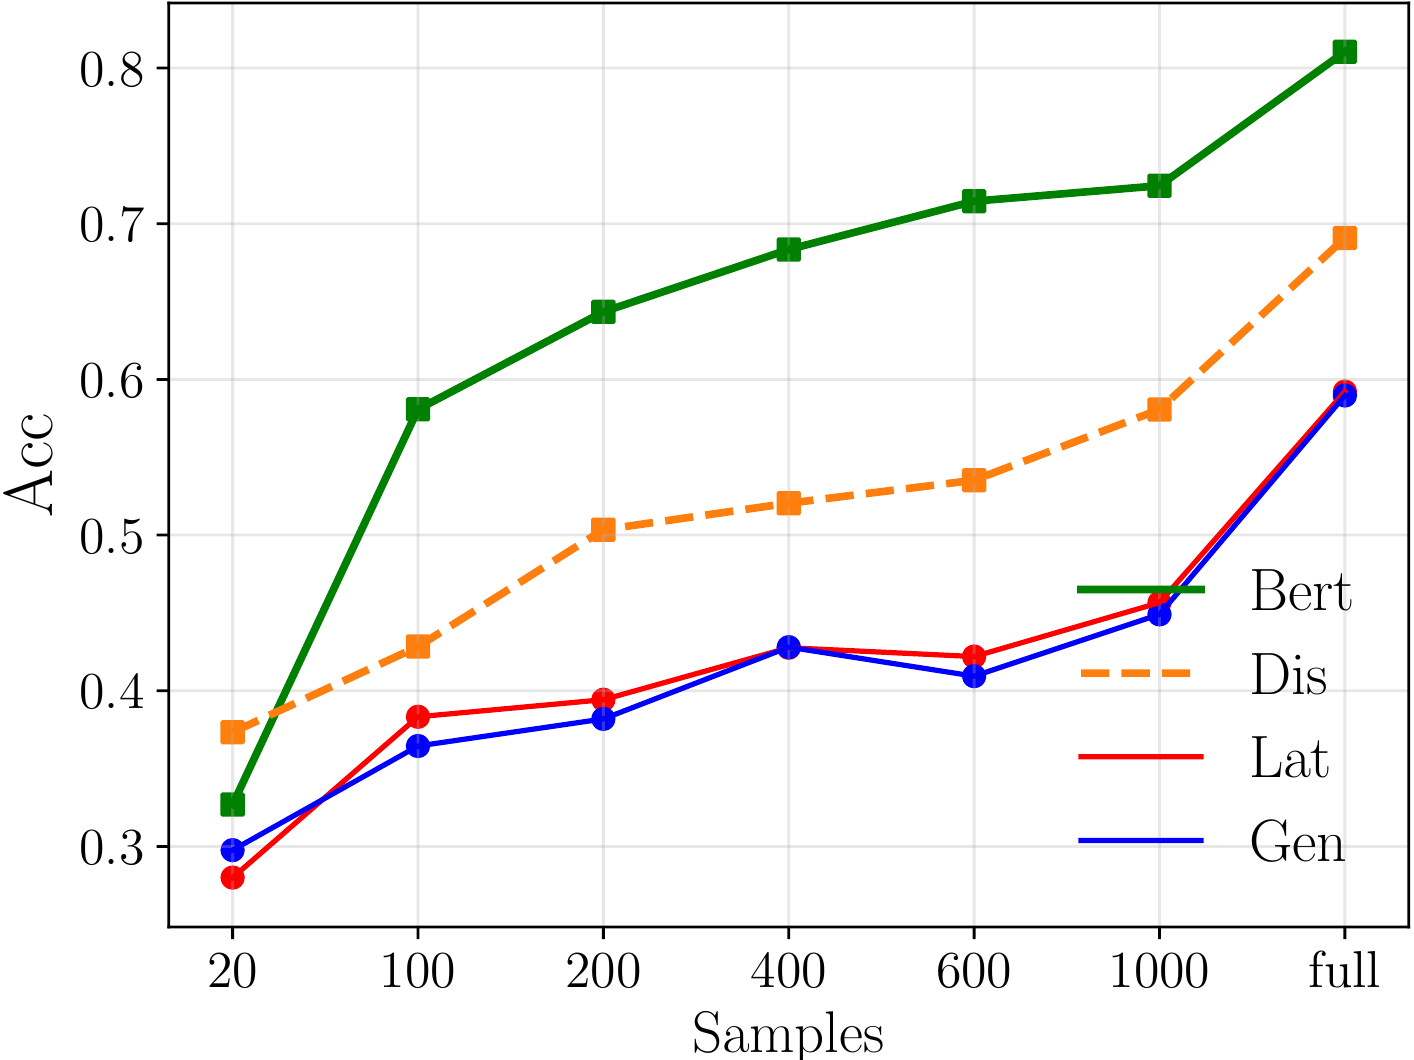}
%   \caption{Original Code }
%   \label{fig:model}
% \end{figure*}
    % \begin{table}[]
    %     \centering
    %     \begin{tabular}{l|ccc}
    %     \specialrule{.1em}{.05em}{.05em} 
    %     Genre     & Context Aware & Bert    &Humans \\ \hline
    %     blog      & 70.3       &\textbf{72.03} & 72.9 \\
    %     email     & 71.5       &\textbf{73.84} & 67.0 \\
    %     essays    & 64.1       &\textbf{66.99} & 64.6 \\
    %     ficlets   & 68.8       &\textbf{75.14}  & 81.7 \\
    %     fiction   & 72.1       &\textbf{77.52}  & 76.7 \\ 
    %     gov-docs  & 68.9       &\textbf{72.52} & 72.6\\
    %     jokes     & 75.0       &\textbf{77.11} & 82.0\\
    %     journal   & 66.4       &\textbf{68.75} & 63.7\\
    %     letters   & 71.2       &\textbf{72.01} & 68.0\\
    %     news      & 72.7       &\textbf{75.20} & 78.6\\
    %     technical & 60.5       &\textbf{61.72}& 54.7\\
    %     travel    & 53.6       &\textbf{68.54} & 48.9\\
    %     wiki      & 60.6       &\textbf{63.04} & 69.2\\
    %     \specialrule{.1em}{.05em}{.05em} 
    %     \end{tabular}
    %     \caption{Cross-genre Classification F-1 Scores by Genre on the Training Set of MASC+Wiki.}
    %     \label{cross-genre result by genre}
    % \end{table}
    
    % \begin{figure}[t!]
%   \centering
%   \includegraphics[width=0.9\linewidth]{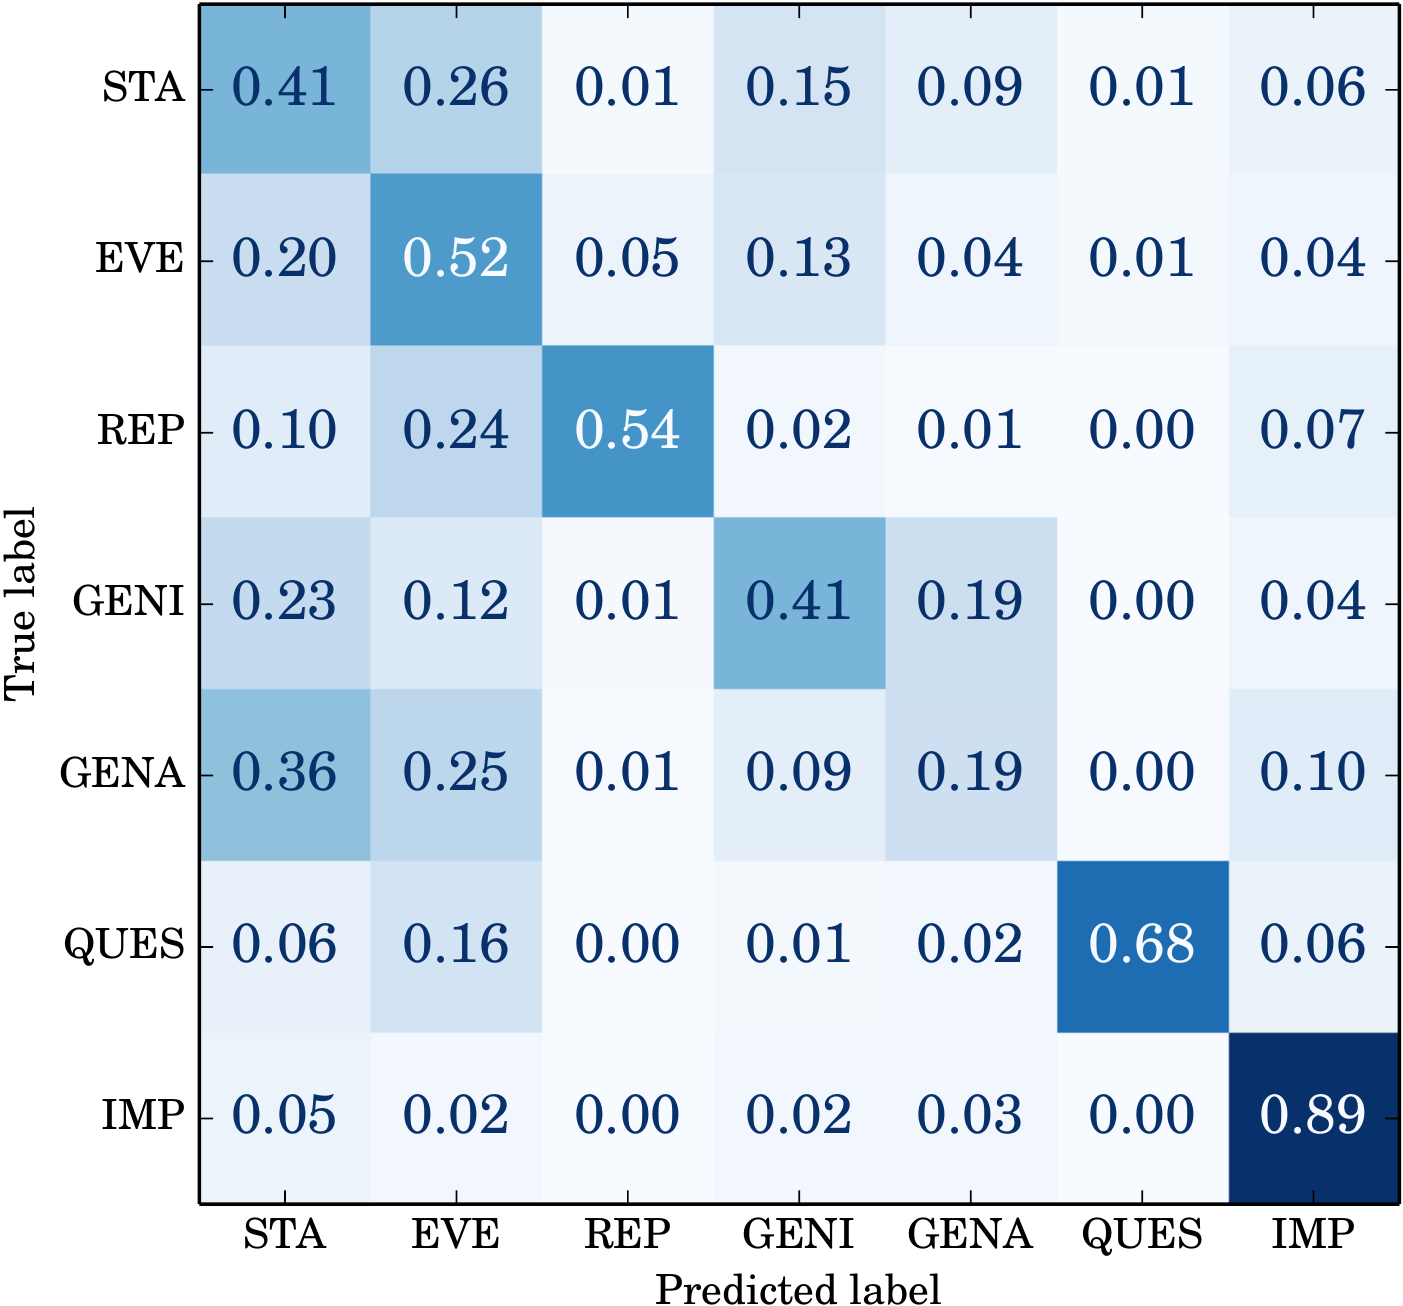}
%   \caption{confusion matrix for test dataset. 20 samples}
%   \label{fig:conf_test_20}
% \end{figure}

% \label{sec:method}

There are other similar tasks such as aspectual class of verbs in context
\ForMR{This paragraph should be revised}
prediction~\citep{friedrich-palmer-2014-automatic}, fine-grained entity type classification (FETC) task~\citep{abhishek-etal-2017-fine}, entity mention classification to predict types from an entity type hierarchy~\citep{karn-etal-2017-end}, fine-grained information status determination which is basically a discourse entity classification task~\citep{rahman-ng-2012-learning}, and supervised identification of generic noun phrases~\citep{reiter-frank-2010-identifying} which can be employed to improve other tasks like knowledge acquisition.
